# Supplementary material for: Fiber networks amplify active stress
Source: arXiv:1507.05873 ancillary file (2015-07-22)
Supplement: Supplementary file 1 [file Supplement-FiberNetworksAmplifyActiveStress.pdf]

# Supporting Information

## Fiber networks amplify active stress

Pierre Ronceray,<sup>1,\*</sup> Chase Broedersz,<sup>2,3,†</sup> and Martin Lenz<sup>1,‡</sup>

<sup>1</sup>*Univ. Paris-Sud; CNRS; LPTMS; UMR 8626, Orsay 91405 France.*

<sup>2</sup>*Lewis-Sigler Institute for Integrative Genomics and Joseph Henry Laboratories of Physics, Princeton University, Princeton, NJ 08544, USA*

<sup>3</sup>*Arnold-Sommerfeld-Center for Theoretical Physics and Center for NanoScience, Ludwig-Maximilians-Universität München, Theresienstrasse 37, D-80333 München, Germany.*

### I. METHODS

#### A. Network energy minimization

Using the network model described in the main text, we investigate the response to localized active forces of the form  $-\mathbf{F}_i \cdot \mathbf{R}_i$  where  $\mathbf{R}_i$  is the position of vertex  $i$  of the network, as illustrated in Fig S1. Summing the associated elastic energy with all fiber stretching and bending contributions, our total Hamiltonian reads:

$$\begin{aligned} \mathcal{H} = & - \sum_{\text{forces } i} \mathbf{F}_i \cdot \mathbf{R}_i \\ & + \sum_{\text{segments } (i,j)} \mu \frac{(\ell_{ij} - 1)^2}{2} \\ & + \sum_{\text{hinges } (i,j,k)} 2 \sin^2 \frac{\theta_{ijk}}{2} \end{aligned} \quad (\text{S1})$$

where  $\ell_{ij}$  is the length of the segment  $(i, j)$  linking vertices  $i$  and  $j$ ,  $\theta_{ijk}$  is the angle formed between two consecutive segments  $(i, j)$  and  $(j, k)$ , and  $\mathbf{R}_i$  is the position

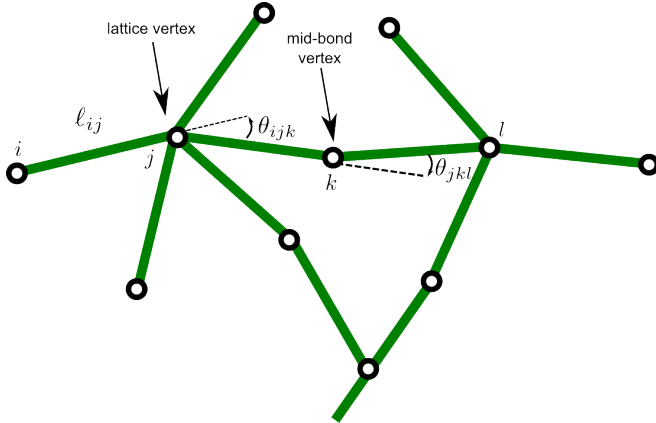

**Figure S1** Schematic representation of the lattice model. The mid-bond vertices allow buckling of individual bonds.

\* pierre.ronceray@u-psud.fr

† c.broedersz@lmu.de

‡ martin.lenz@u-psud.fr

of vertex  $i$  at which the force  $\mathbf{F}_i$  is applied. We consider only the athermal equilibrium response of the system, which is obtained by minimizing the total Hamiltonian of the system using conjugate gradient methods.

#### B. Active stress measurements

The contractility of our active networks is quantified by the value of its macroscopic active stress. To quantify this stress, we use a framework previously developed by us and suited for the analysis of random discrete networks with next-nearest neighbor interactions [1]. This framework includes different prescriptions for systems with fixed and periodic boundary conditions.

For fixed boundary conditions, we compute the system's active stress tensor  $\sigma^{\mu\nu}$  from the forces exerted by the network on its boundaries:

$$\sigma^{\mu\nu} = -\frac{1}{V} \sum_{\text{boundary sites } i} f_i^\mu r_i^\nu, \quad (\text{S2})$$

where the sum runs over the network's boundary sites with positions  $\mathbf{r}_i$ ,  $\mathbf{f}_i$  is the force exerted by the network on the boundary at site  $i$ , and  $V$  is the volume of the system. Note that  $\sum f_i^\mu r_i^\nu$  is in fact the force dipole tensor associated with these boundary forces. In the large length scale limit our active stress tensor  $\sigma^{\mu\nu}$  is exactly identical to the active stress tensor appearing in hydrodynamic active gel theories [2–4].

For periodic boundary conditions (used in Fig. 4 of the main text), we use the so-called mean-stress theorem

$$\sigma^{\mu\nu} = \frac{\Sigma^{\mu\nu}}{V} - \frac{D_{\text{loc}}^{\mu\nu}}{V}, \quad (\text{S3})$$

where  $D_{\text{loc}}^{\mu\nu} = \sum_i F_i^\mu R_i^\nu$  is the force dipole tensor associated with the active forces and  $\Sigma^{\mu\nu} = \sum_{i,j} \sigma_{(i,j)}^{\mu\nu}$  is total stress inside the system, given as a function as the discrete stress  $\sigma_{(i,j)}^{\mu\nu}$  associated with bond  $(i, j)$  [1]. Numerical computations of the active stress from Eq. (S3) are straightforward, as both  $D_{\text{loc}}^{\mu\nu}$  and  $\Sigma^{\mu\nu}$  are readily accessible local quantities.

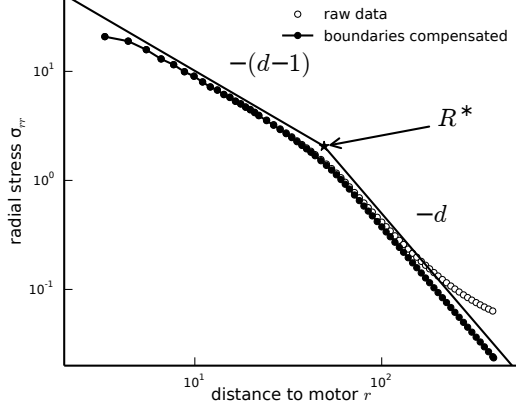

**Figure S2** Compensation of the effect of the fixed boundaries of the system on the spatial distribution of radial stresses.

### C. Measurements of the rope-like region radius

Our definition of the radius  $R^*$  of the rope-like region surrounding an isolated active unit relies on the identification of the crossover of the radial stress  $\sigma_{rr}(r)$  between rope-like and linear stress propagation [Eqs. (5-6) of the main text]. We measure  $\sigma_{rr}(r)$  by performing a virtual “cut” of the system in a circular (or spherical in three dimensions) shell, and averaging the radial components of the stress (including the bending tension) of all fibers that cross this shell. To this end, we use the discrete stress definition introduced in Ref. [1].

The identification of the crossover length is complicated by the fact that the linear regime is not a pure scaling regime. Indeed, it is affected by the boundary conditions of the system. For an isotropic elastic continuum with spherical symmetry, the generic solution to the linear elastic equations for the radial displacement  $u_r(r)$  is:

$$u_r(r) = Ar^{-(d-1)} + Br \quad (\text{S4})$$

where  $d$  is the space dimension, and the constants  $A$  and  $B$  are set by the boundary conditions. The radial stress thus reads

$$\sigma_{rr} = -2d\mu Ar^{-d} + 2\mu \frac{1+\nu}{1-(d-1)\nu} B \quad (\text{S5})$$

where  $\mu$  is the shear modulus and  $\nu$  is the Poisson ratio of the material. In the case of an infinite system,  $B = 0$  and the linear regime is a pure scaling regime  $\sigma_{rr} \propto r^{-d}$ . However, in a finite system, any choice of boundary conditions will lead to a finite value for  $B$ , thus perturbing the scaling regime and complicating the estimation of  $R^*$  (raw value of  $\sigma_{rr}(r)$  in Fig.S2).

In the case of fixed boundary conditions, as in Fig. 3 of the main text, we have  $B = -A/R^d$ , where  $R$  is the

radius of the system. Besides, the Poisson ratio of elastic fiber networks is easily measured, and we numerically find that it is independent of the precise geometry and connectivity of the network: in  $d = 2$ ,  $\nu = 3/5$ , and in  $d = 3$ ,  $\nu = 5/13$  (note that these values do not correspond to actual experimental Poisson ratios, but only to idealized fiber networks, and are exact for regular networks). We can thus extrapolate the infinite-system value of the radial stress by subtracting the part due to the fixed boundaries. To avoid issues associated with bonds that intersect the system’s boundary, we measure the radial stress at a radius  $R_1$  slightly smaller than  $R$ , and compute the corrected “infinite system” stress as a function of our finite-size “raw” measurement using the formula:

$$\sigma_{rr}^{(\text{infinite})}(r) = \sigma_{rr}^{(\text{raw})}(r) - \frac{R_1^d}{R_1^d + gR^d} \sigma_{rr}^{(\text{raw})}(R_1) \quad (\text{S6})$$

where  $g = d - d^2\nu/(1+\nu)$ . Interestingly, in both  $d = 2$  and  $d = 3$  we find  $g = 1/2$ . The corrected stress exhibits a clear scaling regime in the far-field, as demonstrated in Fig. S2, which can then be used to clearly define the rope-like radius  $R^*$ .

### D. Experimental data

As shown in Table 1 of the main text, our predictions on stress amplification are quantitatively supported by a range of experiments in  $d = 2$  and  $d = 3$  in reconstituted cytoskeletal as well as extracellular networks. Here we detail the estimates leading to the figures given in the main text.

Our first example (“system I” in the main text) illustrates the linear regime (Fig. 4b, g of the main text) in three-dimensional actomyosin. In Ref. [5], a crosslinked actin network with mesh size  $\xi = 200$  nm is populated by myosin thick filaments of size  $R_0 = 1\mu\text{m}$  each comprising  $\simeq 300$  myosin heads. Each head actively exerts a  $f = 4$  pN force 2% of the time [6]. Of these 300 heads, half pull in each direction. Furthermore, we use the simplifying assumption that the myosin thick filament is uniformly decorated with motor heads, and thus the average span of the force dipole is  $R_0/2$ . This results in a local force dipole  $\mathcal{D}_{\text{loc}} = -150 \times R_0/2 \times f \times 2\%$  and each thick filament as a whole exerts a typical force  $F = \mathcal{D}_{\text{loc}}/R_0 \simeq 6$  pN on the network. Actin filaments have a persistence length  $\ell_p \simeq 10\mu\text{m}$ , implying a buckling force  $F_b \approx k_B T \ell_p / \xi^3 = 50$  pN for a single network bond. As a result, the active unit force is too small to induce filament buckling, and we thus expect linear force transmission in this experiment. Hence  $\sigma_{\text{th}} = -\rho \mathcal{D}_{\text{loc}} = \rho F R_0 \simeq 12$  Pa, where we used  $\rho = 2\mu\text{m}^{-3}$ . This number is in very good agreement with the estimation  $\sigma_{\text{exp}} \simeq 14$  Pa of the macroscopic stress in Ref. [5].

Our second example (“system II” in the main text) illustrates force-controlled amplification in two-dimensional actomyosin networks (Figs. 4c, g of the

main text). Reference [7] reports measurements based on doublets of giant unilamellar lipid vesicle where the active stresses generated by a membrane-supported two-dimensional actomyosin sheet competes with the tension of a bare lipid membrane to set the angle at which the sheet and the bare membrane meet. This novel measurement technique reveals that the active stresses generated by thick filaments ( $F \simeq 6$  pN as above) in a two-dimensional actin network ( $\xi = R_0 = 1 \mu\text{m}$ ) covering a giant unilamellar vesicle of radius  $r \simeq 10 \mu\text{m}$  are of the same order as the tension of the membrane  $\sigma_{\text{exp}} \approx \sigma_{\text{membrane}} \approx 10^{-6}$ - $10^{-4} \text{ N} \cdot \text{m}^{-1}$  (the vesicles are electroformed and contain a mixture of egg-phosphatidylcholine (EPC) and biotin-PEG lipids). The range of tensions given here are typical values for such vesicles as no direct tension measurement are available in these experiments. The experiments involve an average of three myosin thick filaments per vesicle, implying  $\rho = 3/(4\pi r^2) \simeq 2 \times 10^{-3} \mu\text{m}^{-2}$ . Computing the buckling force as  $F_b \approx k_B T \ell_p / \xi^3 = 0.4$  pN and assuming a stretching-dominated network, we predict a buckling radius  $R^* = R_0 F / F_b = 15 \mu\text{m}$  that is both larger than the mesh size and smaller than the inter-motor spacing  $R_{\text{a.u.}} = \rho^{-1/2} \simeq 20 \mu\text{m}$ , placing this system in the force-controlled amplification regime (Figs. 4c, g of the main text). This yields an amplification factor  $\sigma_{\text{th}}/\sigma_{\text{lin}} = R^*/R_0 \simeq 15$ , and an overall two-dimensional active stress  $\sigma_{\text{th}} = \rho F R^* \simeq 2 \times 10^{-7} \text{ N} \cdot \text{m}^{-1}$ .

Our last example (“system III” in the main text) addresses the density-controlled amplification regime (Figs. 4d, g of the main text). We consider stress

generation in a reconstituted clot comprised of a fibrin network rendered contractile by a concentration  $\rho = 3 \times 10^8 \text{ cells} \cdot \text{mL}^{-1}$  of blood platelets [8]. Atomic force microscopy measurements on individual platelets [9] show that each platelet of size  $R_0 = 2 \mu\text{m}$  exerts a pulling force  $F = 15$  nN, thus yielding a force dipole  $\mathcal{D}_{\text{loc}} = -Fd = -3 \times 10^{-14} \text{ N} \cdot \text{m}$  [9]. The linear prediction for the active stress is thus  $\sigma_{\text{lin}} = -\rho \mathcal{D}_{\text{loc}} \approx 9$  Pa. Comparing this to the experimentally measured active contractile stress  $\sigma_{\text{exp}} = 150$  Pa generated by a blood clot, we thus find a stress amplification factor  $\sigma_{\text{exp}}/\sigma_{\text{lin}} = 17$ . As the microstructure of the fibrin network was not investigated in Ref. [8], we assume that the network essentially consists of single fibrin filaments or of small-diameter fibrin bundles and thus estimate a persistence length  $\ell_p = 0.5 \mu\text{m}$  and a mesh size larger than two hundred nanometers ( $\xi \geq 200 \text{ nm}$ ) [10]. To assess the validity of these estimates, we note that they imply a network shear modulus  $G' \approx 6k_B T \ell_p^2 / \xi^5 \simeq 20$  Pa [11], consistent with the value  $G' = 70$  Pa reported in Ref. [8]. They moreover imply a rope-like region size  $R^* = \xi(F/F_b)^{1/2} \geq 70 \mu\text{m}$  (with  $F_b \approx k_B T \ell_p^2 / \xi^3$ ), larger than the inter-cell distance  $R_{\text{a.u.}} = \rho^{-1/3} \simeq 15 \mu\text{m}$ . The rope-like regions of neighboring cells thus interpenetrate, implying density-controlled amplification. In this regime, we predict a contractile stress  $\sigma_{\text{th}} \simeq 70$  Pa and a stress amplification factor  $\sigma_{\text{th}}/\sigma_{\text{lin}} = R_{\text{a.u.}}/R_0 \simeq 8$ , in order of magnitude agreement with the experimental result. Note that as system III is deep in the density-controlled regime, this prediction is insensitive to our precise estimates of  $\ell_p$  and  $\xi$ .

- 
- [1] P. Ronceray and M. Lenz, *Soft Matter* **11**, 1597 (2015).
  - [2] F. Jülicher, K. Kruse, J. Prost, and J.-F. Joanny, *Phys. Rep.-Rev. Sec. Phys. Lett.* **449**, 3 (2007).
  - [3] J.-F. Joanny and J. Prost, *HFSP J.* **3**, 94 (2009).
  - [4] J. Prost, F. Jülicher, and J.-F. Joanny, *Nat. Phys.* **11**, 111 (2015).
  - [5] G. H. Koenderink, Z. Dogic, F. Nakamura, P. M. Bendix, F. C. MacKintosh, J. H. Hartwig, T. P. Stossel, and D. A. Weitz, *Proc. Natl. Acad. Sci. U.S.A.* **106**, 15192 (2009).
  - [6] S. S. Rosenfeld, J. Xing, L.-Q. Chen, and H. L. Sweeney, *J. Biol. Chem.* **278**, 27449 (2003).
  - [7] J. Lemi re, M. Bussonnier, T. Betz, C. Sykes, and K. Carvalho, “Cell-sized liposome doublets reveal active cortical tension build up,” (2015), to appear.
  - [8] C. J. Jen and L. V. McIntire, *Cell Motil.* **2**, 445 (1982).
  - [9] W. A. Lam, O. Chaudhuri, A. Crow, K. D. Webster, T.-D. Li, A. Kita, J. Huang, and D. A. Fletcher, *Nat. Mater.* **10**, 61 (2011).
  - [10] C. Storm, J. J. Pastore, F. C. MacKintosh, T. C. Lubensky, and P. A. Janmey, *Nature* **435**, 191 (2005).
  - [11] C. P. Broedersz and F. C. MacKintosh, *Rev. Mod. Phys.* **86**, 995 (2014).

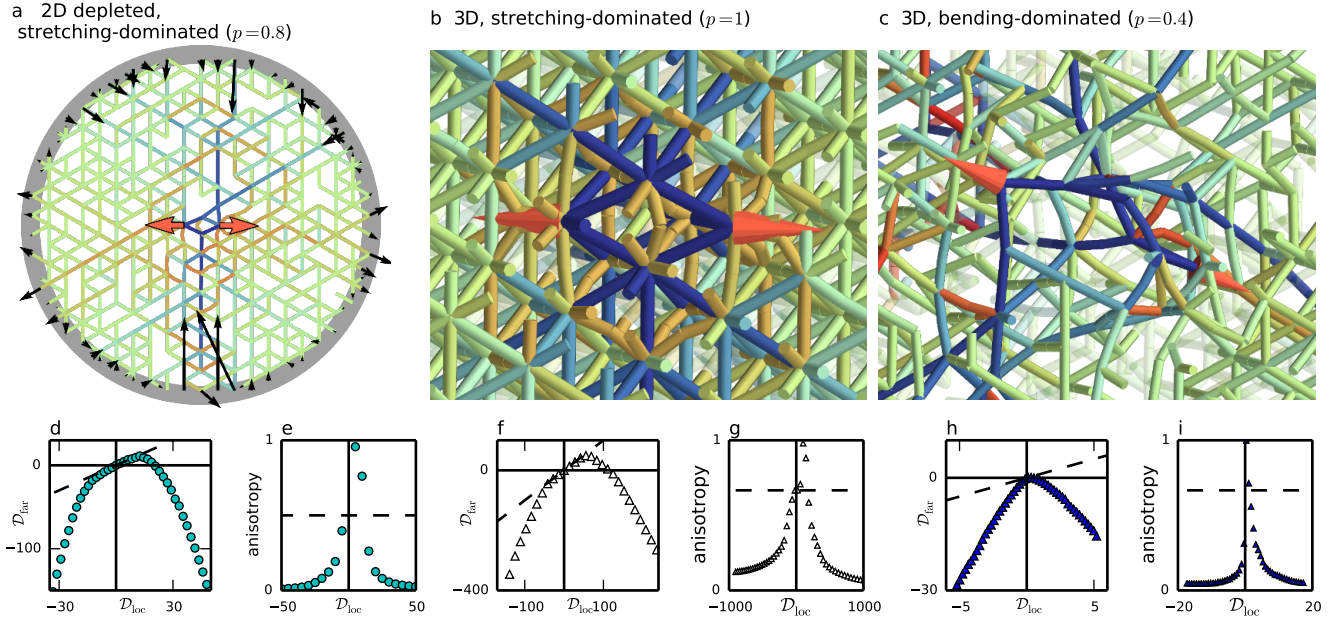

**Figure S3** Rectification, amplification and isotropization effects are generic features of force transmission in fiber networks. **a-c.** Illustration of the rectification effect in response to an extensile force dipole in various networks. Because compressed segments buckle (red bonds), only tensile stresses (blue bonds) are propagated to the far-field. **d, f, h.** The far-field dipole becomes large and contractile for large local force dipoles of either sign. **e, g, i.** The anisotropy of the far-field stress vanishes for large local force dipoles.

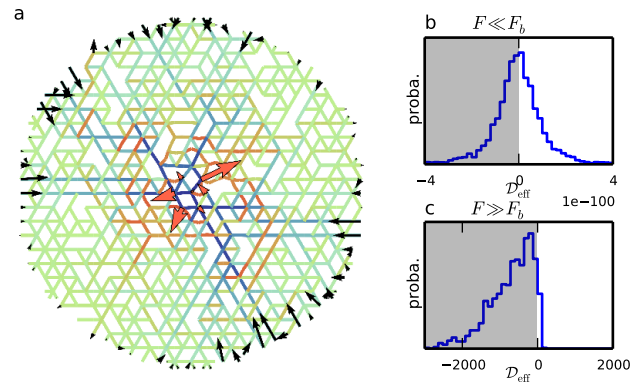

**Figure S4** Rectification of arbitrary local force distributions into far-field contractility. We consider systems where random forces are applied in a small area of 7 lattice vertices, with the constraint that the total force and torque vanish. By symmetry, the resulting average local force dipole is equal to zero. **a.** Typical configuration, showing rectification at large forces. **b.** The distribution of the effective dipole measured at the boundary in the linear limit ( $F \ll F_b$ ). As expected, the distribution is centered around zero, and the average effective dipole thus vanishes. **c.** In the large force limit, effective dipoles are overwhelmingly contractile (95% of cases), demonstrating the generality of the rectification effect. Here  $p = 0.8$ .

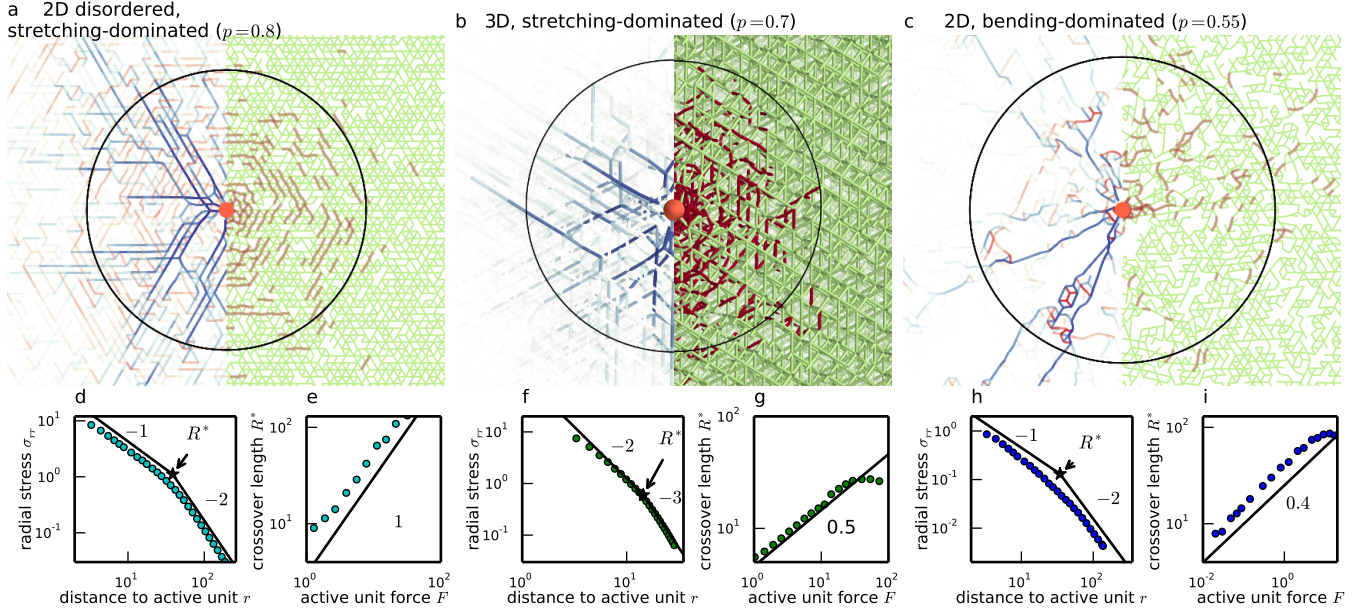

**Figure S5** The force transmission mechanism presented in the main text is insensitive to the specific choice of parameters of the system, and in particular to the choice of the depletion parameter  $p$  characterizing the connectivity of the network. **a-c:** A localized, isotropically pulling active unit (red circle of radius  $R_0 = 1.95$ ) induces stress lines (left side of each panel, blue=tension and red=compression) and buckling (right side of each panel, in red; non-buckled bonds are green) in the surrounding fiber network. Black circle: radius  $R^*$  of the rope-like region. Panel **b** shows a slice of a 3D system. **d, f and h:** Decay of the average radial stress in the network as a function of the distance to the active unit. **e, g and i:** The exponent  $\alpha$  that relates the rope-like radius  $R^*$  to the active force  $F$  depends only on the elasticity regime—stretching- or bending-dominated—and not on the specific value of  $p$ . Indeed,  $\alpha = 1/(d - 1)$  in stretching-dominated networks (panels **e** and **g**), and the 2D anomalous exponent in bending-dominated networks  $\alpha = 0.4$  is reproduced for a lower connectivity than in the main text (panel **i**). Results obtained in a circular (spherical) network of radius 200 (33) with fixed boundaries and averaged over 100 samples for disordered networks..
